# Supplementary material for: Revisiting Granular Models of Firm Growth
Source: arXiv:2404.15226 source file (2024-06-02)
Supplement: Supplementary file 1 [file appendix.tex]

%!TEX root = ./paper.tex 

\section{Sum of $k$ Laplace variables} % (fold)
\label{app:laplace}

Consider the random variable $Y_k = \sum_{i=1}^k X_i/\sqrt{2k}$ where the $X_i$ variables have a Laplace distribution with density
\begin{equation}\label{eq:laplace}
p(x) = \frac{1}{2}\exp(-\abs{x}).
\end{equation}

It is easy to see that this variable is centred and has unit variance, as $\mathbb{E}\left[Y_k\right]=\sqrt{k}\mathbb{E}\left[X_i\right]=0$ and $\mathbb{E}\left[Y_k^2\right]= \frac{\mathbb{E}\left[X_i^2\right]}{2}=1$.

To compute the density of $Y_k$ we will compute its characteristic function $\mathbb{E}\left[\exp\left(\iu t Y_k\right)\right]$, which is none other than the Fourier transform of its density. It can be computed in terms of the characteristic function of the Laplace random variables, obtained by a Fourier transform on the expression in Eq~\eqref{eq:laplace}, as:

\begin{equation}\label{eq:characteristic_function}
\phi_X(t)= \frac{1}{2} \int \dint x~ e^{\iu tx - \abs{x}}= \frac{1}{1+t^2}.
\end{equation}

The characteristic function of $Y_k$ can then be easily written using this function, 
\begin{equation}\label{eq:characteristic_Y}
\phi_{Y_k}(t) = \left[\phi_X\left(\frac{t}{2k}\right)\right]^k = \frac{2^k k^k}{\left(2k+t^2\right)^k}.
\end{equation}

To find the density it is therefore only necessary to invert this transformation.

\subsection{Computing the density for $Y_k$} % (fold)
\label{sub:computing_the_density_for_}

To find the density of $Y_k$, $g_k(y)$, we compute the inverse Fourier transform of its characteristic function, i.e.:

\begin{equation}\label{eq:fourier_inv}
\begin{split}
g_k(y) &=\frac{2^kk^k}{2 \pi} \int \dint t~ \frac{e^{-\iu t y}}{\left(2k+t^2\right)^k}\\
&=\frac{2^kk^k}{2\pi} \int_{\mathcal{C}} \dint z~ f(z)
\end{split}
\end{equation}
with $f(z)=\frac{e^{-\iu z y}}{\left(2k+z^2\right)^k}=\frac{e^{-\iu z y}}{\left(z-\iu\sqrt{2k}\right)^k \left(z+\iu\sqrt{2k}\right)^k}$.

This computation can be done via a complex-plane integral along a contour $\mathcal{C}$ running from $-R$ to $R$ and then around the half-circle centred at the origin and of radius $R>\sqrt{2k}$. The contour is chosen so that it encloses $-\iu\sqrt{2k}$ if $y>0$ and $\iu\sqrt{2k}$ if $y<0$, and then the limit $R\to\infty$ is taken. See Figure~\ref{fig:contour} for an illustration for $y>0$.

\begin{figure}[tb]
    \centering
    \includegraphics[width=8cm]{figures/semicircle.pdf}
    \caption{Example of the contour taken in the case $y>0$.}
    \label{fig:contour}
\end{figure}

In this case, the function $f(z)$ has a pole of order $k$ at $z=-\iu$, of residue

\begin{equation}\label{eq:residue_1}
\mbox{Res}_{-\iu\sqrt{2k}}(f) = \frac{1}{(k-1)!}\lim_{z\to -\iu\sqrt{2k}} \frac{\partial^{(k-1)}}{\partial z^{(k-1)}}\left(\frac{e^{-\iu z y}}{\left(z-\iu\sqrt{2k}\right)^k }\right). 
\end{equation}

To compute the derivative, we apply the generalized Leibniz' rule:
\begin{equation}\label{eq:leib_rule}
\frac{\partial^{(k-1)}}{\partial z^{(k-1)}}\left(\frac{e^{-\iu z y}}{\left(z-\iu\sqrt{2k}\right)^k }\right)= \sum_{l=0}^{k-1}\binom{k-1}{l}\frac{\partial^l}{\partial z^l}\left(e^{-\iu z y}\right)\frac{\partial^{(k-1-l)}}{\partial z^{(k-1-l)}} \left((z-\iu\sqrt{2k})^{-k}\right),
\end{equation}
which then allows for an explicit computation of the residue in Eq.~\eqref{eq:residue_1}:
\begin{equation}\label{eq:full_residue}
\mbox{Res}_{-\iu}(f)= \iu\frac{1}{\left(k-1\right)!}\sum_{l=0}^{k-1}\binom{k-1}{l} \left(2\sqrt{2k}\right)^{l+1-2k} \frac{(2k-2-l)!}{(k-1)!} y^l e^{-\sqrt{2k}y}.
\end{equation}

Plugging this into $g_k(y)=\frac{(2k)^k}{2\pi}\int_{\mathcal{C}}f=-\iu (2k)^k \mbox{Res}_{-\iu}(f)$, and considering the symmetrical case when $y<0$, we obtain
\begin{equation}\label{eq:full_result}
\begin{split}
g_k(y) &= \frac{2^{-2k}2\sqrt{2k}}{\left(k-1\right)!}\sum_{l=0}^{k-1}\binom{k-1}{l} 2^l \frac{(2k-2-l)!}{(k-1)!} (\sqrt{2k}\abs{y})^l e^{-\sqrt{2k}\abs{y}}.
\end{split}
\end{equation}

One can then check how this behaves on Figure~\ref{fig:lap_sum}, where it is evident that the Laplace cusp is not stable upon aggregation of variables. 

\begin{figure}[tb]
    \centering
    \includegraphics[width=.8\textwidth]{figures/fig_laplace_sum.pdf}
    \caption{Examples of the sum of $k$ Laplace variables for $k=\{1,2,4,8\}$ with a Gaussian for comparison. Note that the Laplace ``cusp'' is already gone at $k=2$.}
    \label{fig:lap_sum}
\end{figure}

\subsection{Extension to sums of correlated Laplace variables} % (fold)
\label{sub:extension_to_sums_of_correlated_laplace_variables}
Suppose now that we want to compute the distribution of the sum of two Laplace random variables $X_1$ and $X_2$, with $\mathbb{E}(X_1X_2)=\rho$, and where both variables have the density given in Eq.~\eqref{eq:laplace}.

To tackle this problem, we first prove a preliminary result, which is that the variables $X$ can be represented as a superposition of Gaussian random variables with variances distributed according to an exponential distribution, namely

\begin{equation}\label{eq:lap_super}
X \overset{\text{law}}{=} \mathbb{E}_{\sigma}\left[Y_{\sigma}\right] ,
\end{equation}
where the distribution of $Y_{\sigma}$ and of $\sigma$\footnote{Mind that $\sigma$ is the square root of the variance, and that it is only its square that is distributed exponentially.} are given by

\begin{equation}\label{eq:densities}
p_{Y_{\sigma}}(y) = \frac{1}{\sqrt{2\pi\sigma^2}} e^{-y^2/2\sigma^2},\quad p_{\sigma}(\sigma)= \sigma e^{-\sigma^2/2}\mathbf{1}_{\sigma>0}.
\end{equation}

To prove this, one need only compute the characteristic function of $X$ as
\begin{equation}\label{eq:characteristic_function_superp}
\begin{split}
\phi_{X}(t) &= \int_{0}^\infty\dint \sigma ~ \sigma e^{-\sigma^2/2}\left[\int \frac{\dint y}{\sqrt{2\pi \sigma^2}}\exp\left(-\frac{y^2}{2\sigma^2}+ity\right)\right]\\
&=\int_{0}^\infty\dint \sigma~ \sigma \exp\left(-\frac{\sigma^2}{2}\left(1+t^2\right)\right)\\
&= \frac{1}{1+t^2},
\end{split}
\end{equation}
which proves our assertion.

We can now generalize to try to find the sum of $k$ correlated Laplace variables. To do this, we will consider the sum $\sum_{l=1}^{k}\sigma_l Y_l$ where $Y_0$ is Gaussian and
\begin{equation}\label{eq:ar1}
Y_{l} = \rho Y_{l-1} + \sqrt{1-\rho^2} \eta_l, 
\end{equation}
with $\eta_l$ a Gaussian white noise of unit variance and $\sigma_l$ distributed according to the density in Eq.~\eqref{eq:densities}. One sees that in this case the variables $\sigma_l Y_l$ are Laplace-distributed, with $\Cor(\sigma_l Y_l, \sigma_{l+1}Y_{l+1})=2\rho $. 

For $k=2$ the sum is 
\begin{equation}\label{eq:s2}
 S_2 = \sigma_1Y_1 + \sigma_2 Y_2 = \sigma_1 Y_1 + \rho \sigma_2 Y_1 + \sigma_2 \sqrt{1-\rho^2}\eta_2,
 \end{equation} 
 which, owing to the Gaussian nature of $Y_1,Y_2$ and $\eta_2$ can be written as
 \begin{equation}\label{eq:rewriting}
 S_2 = \sqrt{\left(\sigma_1 + \rho\sigma_2\right)^2 + \sigma_2^2 \left(1-\rho^2\right)}\xi,
 \end{equation}
 with $\xi$ Gaussian with unit variance. 

 We can then compute the characteristic function of $S_2$ given $(\sigma_1,\sigma_2)$:

\begin{equation}
    \phi_2(t,\sigma_1,\sigma_2)=\mathbb{E}\left[\exp\left(\iu t S_2\right) |\sigma_1, \sigma_2\right] = \exp\left(-\frac{\left(\sigma_1 + \rho\sigma_2\right)^2 + \sigma_2^2 \left(1-\rho^2\right)}{2}t^2\right).
\end{equation}

This last expression can then be averaged using the distributions of $\sigma_1$ and $\sigma_2$ to obtain the characteristic function of $S_2$:

\begin{equation}\label{eq:nasty_int}
\begin{split}
\phi_2(t) &= \int_{0}^{\infty}\dint \sigma_1~\sigma_1e^{-\frac{\sigma_1^2}{2}}\int_{0}^{\infty}\dint \sigma_2~\sigma_2e^{-\frac{\sigma_2^2}{2}}\phi_2(t,\sigma_1,\sigma_2)\\
&= \int_{0}^{\infty}\dint \sigma_1 \int_{0}^{\infty}\dint \sigma_2~~\sigma_1\sigma_2 \exp\left(-\frac{1}{2}\Braket{\sigma | \mathbf{A} | \sigma}\right),
\end{split}
\end{equation}
where the matrix $\mathbf{A}= \left( \begin{matrix}
1+t^2 & t^2\rho \\ t^2\rho & 1+t^2
\end{matrix}  \right)$ has two eigenvectors, $\ket{u} = \frac{1}{\sqrt{2}}\left(1,1\right)$ corresponding to eigenvalue $\lambda_1 = 1+t^2\left(1-\rho\right)$  and $\ket{v}=\frac{1}{\sqrt{2}}(1,-1)$ corresponding to  $\lambda_2 = 1+t^2\left(1+\rho\right)$. The dependence in $t$ of $\lambda_1,\lambda_2$ is implicit.

Next, we substitute $u=\frac{\sqrt{2}}{2}\left(\sigma_1+\sigma_2\right)$ and $v=\frac{\sqrt{2}}{2}\left(\sigma_1-\sigma_2\right)$ in Eq.~\eqref{eq:nasty_int}, to obtain
\begin{equation}
\begin{split}
\phi_2(t) =& \frac{1}{2}\int\dint v \int \dint u ~\left(u^2-v^2\right)\exp\left(-\lambda_1\frac{u^2}{2}-\lambda_2\frac{v^2}{2}\right)\mathbf{1}_{u+v>0}\mathbf{1}_{u-v>0} \\
=& \frac{1}{2}\int\dint v \int \dint u~u^2 \exp\left(-\lambda_1\frac{u^2}{2}-\lambda_2\frac{v^2}{2}\right)\mathbf{1}_{u+v>0}\mathbf{1}_{u-v>0}\\
&+ \frac{1}{2}\int\dint v \int \dint u~v^2 \exp\left(-\lambda_1\frac{u^2}{2}-\lambda_2\frac{v^2}{2}\right)\mathbf{1}_{u+v>0}\mathbf{1}_{v-u>0}.
\end{split}
\end{equation}

This integral can be computed explicitly, first by integrating over $v$ and then by setting $w=\sqrt{\frac{\lambda 1}{2}}u$, to get
\begin{equation}\label{eq:nasty_1}
\begin{split}
\int \dint u~e^{-\lambda_1 \frac{u^2}{2}}u^2 \int\dint v~ e^{-\lambda_2 \frac{v^2 }{2}}\mathbf{1}_{u+v>0}\mathbf{1}_{u-v>0} &= 2\sqrt{\frac{\pi}{2\lambda_2}} \int_{0}^{\infty}\dint u~e^{-\lambda_1 \frac{u^2}{2}}u^2 \text{erfc}\left(\sqrt{\frac{\lambda_2}{2}}u\right)\\
&= 4\sqrt{\frac{\pi}{\lambda_2}}\frac{1}{\lambda_1^{3/2}}\int_{0}^{\infty}\dint w~e^{-w^2}w^2 \text{erfc}\left(\sqrt{\frac{\lambda_2}{\lambda_1} w} \right),
\end{split}
\end{equation}
with the last integral giving (see e.g. \cite{Ng_Geller_1969})
\begin{equation}
    \int_{0}^{\infty}\dint w~e^{-w^2}w^2 \text{erfc}\left(\sqrt{\frac{\lambda_2}{\lambda_1} w} \right) = \frac{1}{2\sqrt{\pi}}\left(\arctan\left(\sqrt{\frac{\lambda_1}{\lambda_2}}\right)- \frac{\lambda_1}{\lambda_2+\lambda_1}\sqrt{\frac{\lambda_2}{\lambda_1}}\right).
\end{equation}

Plugging this last expression back into Eq.~\eqref{eq:nasty_1} leads to
\begin{equation}\label{eq:nasty_1_complete}
\begin{split}
\int \dint u~e^{-\lambda_1 \frac{u^2}{2}}u^2 \int\dint v~ e^{-\lambda_2 \frac{v^2 }{2}}\mathbf{1}_{u+v>0}\mathbf{1}_{u-v>0}  &= \frac{2}{\lambda_1^{3/2}\lambda_2^{1/2}}\left(\arctan\left(\sqrt{\frac{\lambda_1}{\lambda_2}}\right)- \frac{\lambda_1}{\lambda_2+\lambda_1}\sqrt{\frac{\lambda_2}{\lambda_1}}\right),
\end{split}
\end{equation}
from which we can give the full expression of the characteristic function $\phi_2(t)$:
\begin{equation}\label{eq:nasty_2}
\phi_2(t)=\frac{\arctan(\sqrt{\lambda_1/\lambda_2})}{\lambda_1^{3/2}\lambda_2^{1/2}}+\frac{\arctan(\sqrt{\lambda_2/\lambda_1})}{\lambda_2^{3/2}\lambda_1^{1/2}}-\frac{1}{\sqrt{\lambda_1\lambda_2}\left(\lambda_1+\lambda_2\right)}\left(\sqrt{\frac{\lambda_2}{\lambda_1}}+\sqrt{\frac{\lambda_1}{\lambda_2}}\right).
\end{equation}

We next study the properties of $p_2(s)$, the distribution of $S_2$, which is but the inverse Fourier transform of $\phi_2$. 
Given that $\abs{\rho}<1$, we can write $\lambda_1(t) = \left(1+t^2\right)\left(1-\frac{t^2}{1+t^2}\rho\right)$ and $\lambda_2(t)=\left(1+t^2\right)\left(1+\frac{t^2}{1+t^2}\rho\right)$, and so the asymptotic behaviour $\phi_2(t)\underset{\abs{t}\gg 1}{\propto}(1+t^2)^{-2}$ is clear. When $\abs{\rho}=1$ however, we have e.g. $\lambda_1=1$ and $\lambda_2 = 1+2t^2$, and as a consequence $\phi_2(t)\sim t^{-3}$ for large $t$.

One can then look at the curvature of the distribution function $p_2(s)$ of the sum $S_2$ defined in Eq.~\eqref{eq:s2}, given by
\begin{equation}
    p_2''(0) = \int \dint t~t^2 \phi(t),
\end{equation}
and see that it behaves as $(1-\abs{\rho})^{-3/2}$. Since this quantity is finite for $\abs{\rho}<1$, it follows that the distribution of $p_2(s)$ cannot have a Laplace cusp at $s=0$, as it would correspond to an infinite curvature.

In general for the case of the sum of $N$ Laplace variables with the correlation structure given in Eq.~\eqref{eq:ar1} one can generalize Eq.~\eqref{eq:nasty_int} with a circulant matrix
\begin{equation}\label{eq:a_matrix}
\mathbf{A} = \left( \begin{matrix}
1+t^2& t^2\rho& \ldots &t^2\rho^{N-2} &t^2\rho^{N-1}\\
t^2\rho& 1+t^2& t^2\rho& &t^2\rho^{N-2}\\
\vdots& t^2\rho& 1+t^2& \ddots& \vdots\\
t^2\rho^{N-2}& & \ddots& \ddots& t^2\rho \\
t^2\rho^{N-1}& t^2\rho^{N-2}& & t^2\rho & 1+t^2
\end{matrix} \right),
\end{equation}
leading to similar, though more complicated, computations.
